# Supplementary material for: M-CTX: Exact and Scalable Spatial Context Retrieval for Trajectory Analytics
Source: arXiv:2606.15244 source file (2026-06-13)
Supplement: Supplementary file 1 [file appendix.tex]

\appendix

\section{Complexity Analysis}
\label{app:theory}

We summarise the asymptotic costs of the three M-CTX operators. The goal
is not to claim a universal optimality result for the full pipeline, but
to show that each replacement removes the avoidable brute-force term in
the reference implementation.

\paragraph*{Static OSM range retrieval.}
The STR-tree bulk-loads $N$ feature MBRs in $O(N\log N)$ time and answers
range queries by traversing page MBRs followed by exact feature-level MBR
filters. The R$^{*}$-tree has the standard logarithmic expected access
behaviour under balanced pages, with worst-case linear degeneration in
pathological layouts. BR-LZ sorts features by Morton key in
$O(N\log N)$, fits $S$ linear segments in $O(N)$, and stores
$\Theta(N+S)=\Theta(N)$ words. With $S=\Theta(\sqrt N)$, the residual-
expanded candidate scan gives the structural query bound
$O(\log N+\sqrt N)$ before the exact output filter
(Section~\ref{ssec:pareto}).

\paragraph*{SDF materialisation.}
For an $H\times W$ grid with $M$ occupied mask pixels, the reference
kernel costs $O(HW\cdot M)$ because it compares every grid cell with every
mask pixel. The Felzenszwalb--Huttenlocher transform computes the exact
Euclidean distance transform in $\Theta(HW)$ time
~\cite{felzenszwalb2004distance}. Since any algorithm that emits the full
field must write $\Omega(HW)$ cells, M-CTX removes the occupancy-dependent
factor and reaches the natural output-size bound for SDF construction.

\begin{table}[t]
\centering
\caption{High-resolution SDF latency (ms/sample). The quadratic kernel
scales with occupancy, while M-CTX remains close to output-size cost.}
\label{tab:sdf-extreme}
\small
\setlength{\tabcolsep}{4pt}
\begin{tabular}{llrrr}
\toprule
Grid & Occupancy & Naive & M-CTX & Speed-up \\
\midrule
$256$ & $1\%$  & $498.8$   & $4.20$ & $119\times$ \\
$256$ & $10\%$ & $4\,060$  & $5.89$ & $689\times$ \\
$512$ & $1\%$  & $5\,434$  & $21.4$ & $254\times$ \\
$512$ & $10\%$ & $54\,920$ & $23.4$ & $\mathbf{2\,343\times}$ \\
\bottomrule
\end{tabular}
\setlength{\tabcolsep}{6pt}
\end{table}

\paragraph*{Streaming neighbour retrieval.}
A B$^{x}$-tree insert costs $O(\log N)$ in the active phase index. Query
processing enumerates Morton key intervals, scans the candidate slice, and
then applies an exact geographic radius filter. The key scan controls
candidate generation, while the radius filter preserves exact recall.
Compared with snapshot rebuilding, the asymptotic advantage is not merely
query latency, but the ability to interleave inserts and queries without
rebuilding the full snapshot.

\paragraph*{Per-anchor workload.}
A context answer must at least read or emit its output: the local SDF
contains $\Omega(g^2)$ cells, the OSM stage must return
$K_{\mathrm{OSM}}$ features, and the neighbour stage must return $k$
vessels. M-CTX therefore removes the avoidable linear scans in the
reference implementation while retaining exact output semantics.

\section{Joint Context Index}
\label{app:jcx}

The main system composes three specialised operators. We also implement an
optional Joint Context Index (JCX) that shares the first spatial
localisation step across them. JCX partitions space into a Morton-cell grid
of depth $B$. Each cell stores the OSM feature MBRs whose centroids fall
inside it, optional coarse SDF metadata, and pointers to AIS records that
are also maintained in the global phase-aware B$^{x}$-tree.

A query enumerates the overlapping cells once and dispatches the resulting
candidate lists to the same exact filters used by the individual
operators. Because the cell enumeration is a superset of the candidates
seen by the specialised indexes, JCX inherits their recall properties. Its
benefit is architectural: it avoids repeating spatial localisation three
times when a deployment wants to co-schedule OSM, SDF, and neighbour
retrieval. We keep JCX optional because the specialised composition is
simpler, easier to audit, and already provides the headline speed-ups.

\section{Additional SDF Precision Results}
\label{app:sdf-precision}

Section~\ref{ssec:storage} reports the storage--accuracy frontier. Here we
show the full precision sweep used to choose that operating point. Each
configuration is evaluated with the pretrained \texttt{lstm\_env\_sdf}
checkpoint on $n=2{,}000$ test anchors.

\begin{table}[t]
\centering
\caption{SDF precision sensitivity. $\Delta$ADE is measured against the
f32 reference representation.}
\label{tab:sdf-prec}
\small
\setlength{\tabcolsep}{4pt}
\begin{tabular}{llrr}
\toprule
Level & Description & SDF MAE (m) & $\Delta$ADE (m) \\
\midrule
L0 & f32 reference              & $0.0$    & $0.000$ \\
L1 & f16 storage                & $0.0$    & $0.000$ \\
L4 & $64^2$ resolution          & $0.6$    & $+0.008$ \\
L5 & $32^2$ resolution          & $1.4$    & $+0.020$ \\
L6 & 8-bit quantisation         & $52.5$   & $-0.003$ \\
L3 & narrow band $\pm500$\,m    & $4\,175$ & $+66.5$ \\
L2 & narrow band $\pm1$\,km     & $3\,697$ & $+103.7$ \\
\bottomrule
\end{tabular}
\setlength{\tabcolsep}{6pt}
\end{table}

\begin{figure}[t]
\centering
\includegraphics[width=0.9\columnwidth]{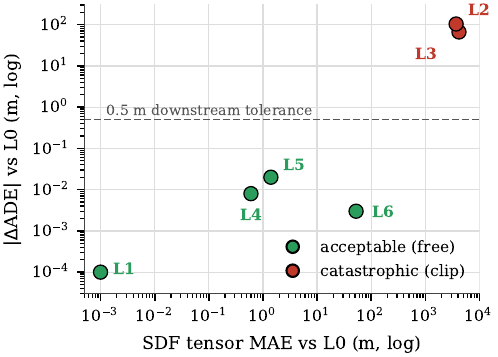}
\caption{ADE penalty versus SDF tensor error. Downsampling and
quantisation are harmless, while narrow-band clipping is not.}
\label{fig:sdf-prec}
\end{figure}

The sweep gives two practical lessons. First, uniform 8-bit quantisation
can introduce a large tensor MAE while leaving ADE unchanged, indicating
that the model uses the coarse SDF gradient rather than exact per-cell
magnitudes. Second, clipping is qualitatively different from compression:
it saturates the long-range distance signal and shifts the feature
distribution seen by the model. This explains why the recommended storage
mode compresses along dtype and resolution, but keeps the full distance
range.

\begin{figure}[t]
\centering
\includegraphics[width=0.8\columnwidth]{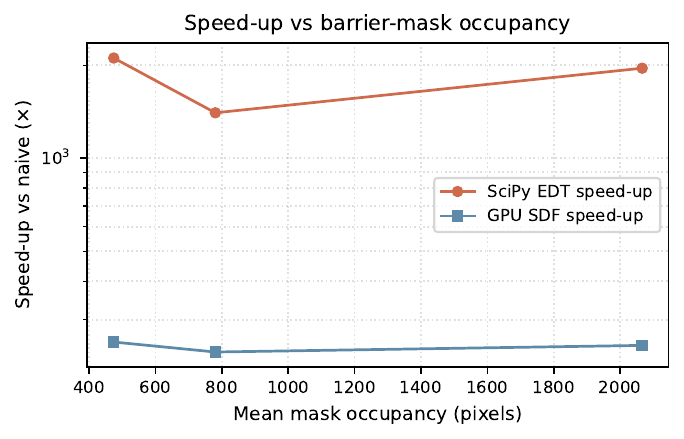}
\caption{SDF speed-up grows with mask occupancy, matching the replacement
of an $O(HW\cdot M)$ kernel by an occupancy-invariant $O(HW)$ transform.}
\label{fig:sdf-occ}
\end{figure}

\section{Extended Scaling and Deployment}
\label{app:extended}

\paragraph*{Hyper-parameter robustness.}
Figure~\ref{fig:ablation} shows the three main hyper-parameter sweeps.
The STR page size has a shallow optimum near $M=16$; BR-LZ degrades
smoothly as the segment count moves away from the default; and the
B$^{x}$-tree phase length changes query latency by less than $4\%$ over
the tested range. The defaults used in the main experiments are therefore
not sensitive tuning points.

\begin{figure}[t]
\centering
\includegraphics[width=0.32\columnwidth]{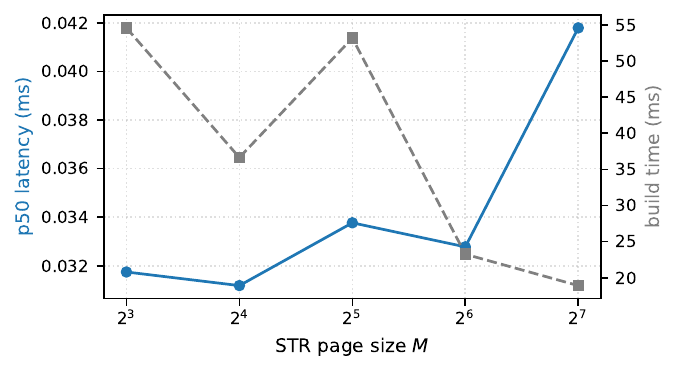}\hfill
\includegraphics[width=0.32\columnwidth]{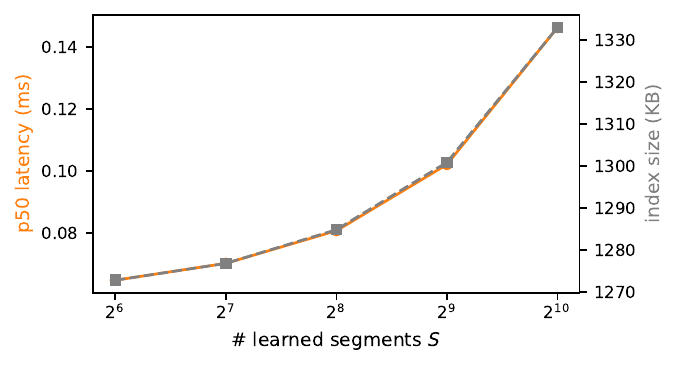}\hfill
\includegraphics[width=0.32\columnwidth]{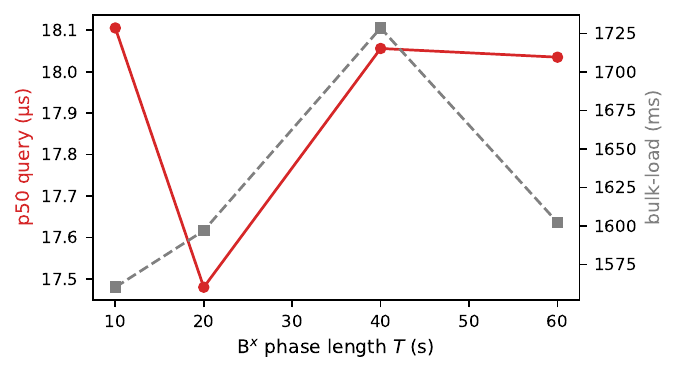}
\caption{Hyper-parameter ablations: STR page size $M$ (left), BR-LZ
segment count $S$ (centre), and B$^{x}$-tree phase length $T$ (right).}
\label{fig:ablation}
\end{figure}

\paragraph*{Space-tiled sharding.}
For multi-worker deployment, M-CTX partitions spatial features into
disjoint tiles and routes each query only to overlapping shards.
Figure~\ref{fig:shard-part} compares two strategies. Morton-rank stripes
balance feature count but create overlapping shard bounding boxes, causing
many queries to touch all shards. A kd-tree median split produces disjoint
spatial cells and keeps routing local.

\begin{figure}[t]
\centering
\includegraphics[width=0.96\columnwidth]{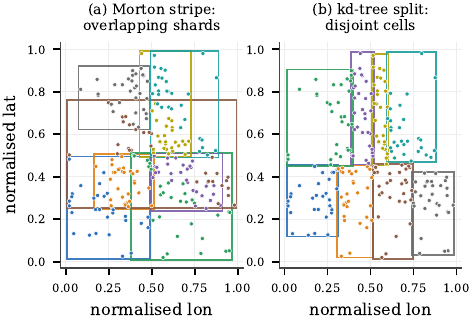}
\caption{Shard partitioning. Morton-rank stripes have overlapping spatial
footprints, while kd-tree median splits produce disjoint spatial cells and
lower routing cost.}
\label{fig:shard-part}
\end{figure}

\begin{figure}[t]
\centering
\includegraphics[width=0.9\columnwidth]{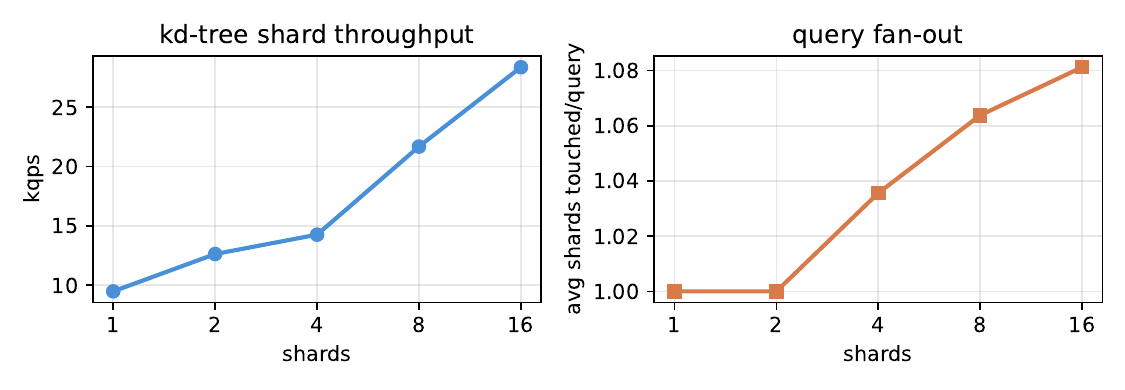}
\caption{Space-tiled shard simulator. Mean shards touched per query stays
below $1.08$, supporting clean partitioning for multi-worker execution.}
\label{fig:shard}
\end{figure}

\paragraph*{Additional cross-region evidence.}
Table~\ref{tab:cross-dataset} repeats the OSM benchmark on the NOAA cache,
which contains more than twice as many features as DMA. The relative
ranking of the exact backends is preserved, and median latency remains
close to the DMA result. Together with the Norway and Piraeus runs, this
supports the claim that M-CTX is not tuned to one coastline distribution.

\begin{table}[t]
\centering
\caption{Cross-dataset OSM benchmark on DMA and NOAA
($r=5$\,km, recall $1.000$).}
\label{tab:cross-dataset}
\small
\setlength{\tabcolsep}{4pt}
\begin{tabular}{llrrr}
\toprule
Dataset & Index & Build (ms) & $p_{50}$ ($\mu$s) & QPS \\
\midrule
DMA  ($40$K) & STR-tree   & $30$  & $\mathbf{65.4}$ & $15$\,k \\
              & LibSpatial & $82$  & $70.9$           & $14$\,k \\
\midrule
NOAA ($90$K) & STR-tree   & $76$  & $\mathbf{78.0}$ & $13$\,k \\
              & LibSpatial & $165$ & $84.0$           & $12$\,k \\
\bottomrule
\end{tabular}
\setlength{\tabcolsep}{6pt}
\end{table}

Across the four real regions, all exact backends maintain recall
$1.000$ without per-region retuning. The regions span roughly two orders
of magnitude in feature count and include open coastlines, fjords, and
dense port geometry, giving a stronger robustness test than a single
national OSM cache.

\section{Reproducibility}
\label{app:repro}

Each reported number is generated from a JSON artefact and aggregated into
a master result table. An audit script re-computes every displayed
speed-up from its source latencies and flags any drift between tables,
figures, and text. A staged runner replays the experiments from a fresh
checkout using completion markers; a clean replay takes approximately
four hours and is dominated by OSM tile loading. The environment uses
Python~3.11 with NumPy, SciPy, PyTorch, Shapely~2, h3-py, DuckDB, and
libspatialindex. Exact package versions and per-table commands are
included with the code release.
